# Supplementary material for: Topological defects in string theory orbifolds with target spaces $\mathbb{C}/\mathbb{Z}_N$ and $S^1/\mathbb{Z}_2$
Source: arXiv:1706.05741 source file (2017-06-18)
Supplement: Supplementary file 3 [file appendix2.tex]

%%%%%%%%%%%%%%%%%%%%%%%%%%%%%%%%%%%%%%%%%%%%%%%%%%%
%
%  New template code for TAMU Theses and Dissertations starting Fall 2016.
%
%
%  Author: Sean Zachary Roberson 
%	 Version 3.16.09 
%  Last updated 9/12/2016
%
%%%%%%%%%%%%%%%%%%%%%%%%%%%%%%%%%%%%%%%%%%%%%%%%%%%

%%%%%%%%%%%%%%%%%%%%%%%%%%%%%%%%%%%%%%%%%%%%%%%%%%%%%%%%%%%%%%%%%%%%%%
%%                           APPENDIX B
%%%%%%%%%%%%%%%%%%%%%%%%%%%%%%%%%%%%%%%%%%%%%%%%%%%%%%%%%%%%%%%%%%%%%

\chapter{\uppercase {A Second Appendix Whose Title Is Much Longer Than The First}}

Text for the Appendix follows.

\begin{figure}[h]
\centering
\includegraphics[scale=.50]{figures/Penguins.jpg}
\caption{Another TAMU figure.}
\label{fig:tamu-fig6}
\end{figure}

\section{Appendix Section}

\section{Second Appendix Section}

\pagebreak{}
